# Supplementary material for: An alternative approach for the determination of mean free paths of electron scattering in liquid water based on experimental data
Source: arXiv:1912.08469 ancillary file (2019-12-18)
Supplement: Supplementary file 1 [file supplement.pdf]

Supporting Information for

# *"An alternative approach for the determination of mean free paths of electron scattering in liquid water based on experimental data"*

Axel Schild, Michael Peper, Conaill Perry, Dominik Rattenbacher, Hans Jakob Wörner

December 18, 2019

## 1 Differential scattering cross sections

In the simulations, differential scattering cross sections (DCS) for elastic $\mathtt{J} = 0 \rightarrow \mathtt{J}' = 0$ scattering are used. These were computed with the programs ePolyScat [1, 2]. ePolyScat calculates scattering properties of electrons at atomic and molecular targets by solving the variational Schwinger equation using a single-center expansion. ePolyScat can be used for relatively high electron kinetic energy (eKE), provided that the inclusion of basis functions with large enough angular momentum quantum numbers is computationally feasible. Due to the single-center expansion, however, the description of the electronic structure of a molecule is necessarily limited compared to a multi-center expansion, where the electronic wavefunction is expanded in a basis set with functions centered at all the nuclei (like e.g. the atom-centered basis sets used in electronic structure calculations of molecules). As input for the calculations with ePolyScat, molecular orbital data from a Hartree-Fock calculation with a cc-pVTZ basis set, generated with Gaussian 09 [3], was used.

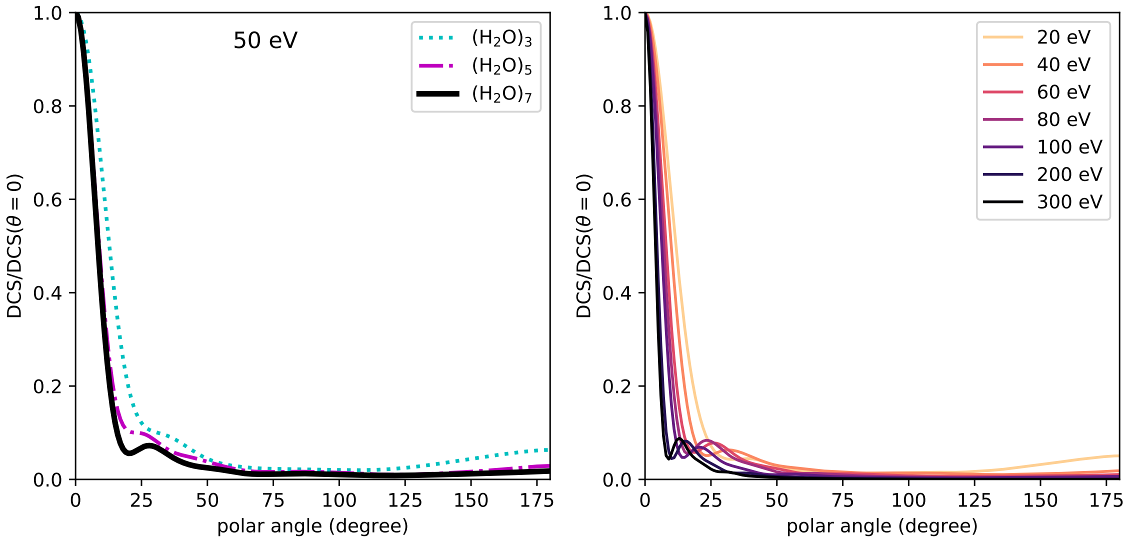


Figure S1: Left: Elastic differential scattering cross sections (DCS) for water clusters $(H_2O)_\mathtt{n}$ with $\mathtt{n} = 3, 5, 7$ calculated with ePolyScat for an electron kinetic energy of 50 eV. For the calculation, Hartree-Fock theory is used. The nuclear configurations for the clusters are the configurations given in [4] of lowest energy with the respective number of water molecules. Right: DCS obtained from ePolyScat for $(H_2O)_7$ clusters, for different kinetic energies of the scattering electron.

We considered water clusters of different sizes and shapes with nuclear configurations taken from the *ab initio* calculations in [4] that have the lowest energy for a given number of water molecules. We use ePolyScat DCS for simulations with an eKE of up to 300 eV. Convergence of the DCS for higher eKE was computationally not feasible.

In the left panel of Figure S1, the calculated DCS are shown for eKE = 50 eV, for water clusters of different sizes. Only the shape of the DCS is relevant for the simulations, not its magnitude, hence the DCS in the figure are scaled to unit magnitude for zero polar angle. It is apparent from the comparison in the figure that there is a convergence of the shape of the DCS with the size of the water clusters. Based on the rapid convergence of the DCS with increasing cluster size, we decided to approximate the DCS of bulk water with that of the water heptamer $(H_2O)_7$. The right

panel of Figure S1 shows the dependence of the DCS on the eKE. It is apparent that the DCS becomes narrower in forward direction with increasing eKE.

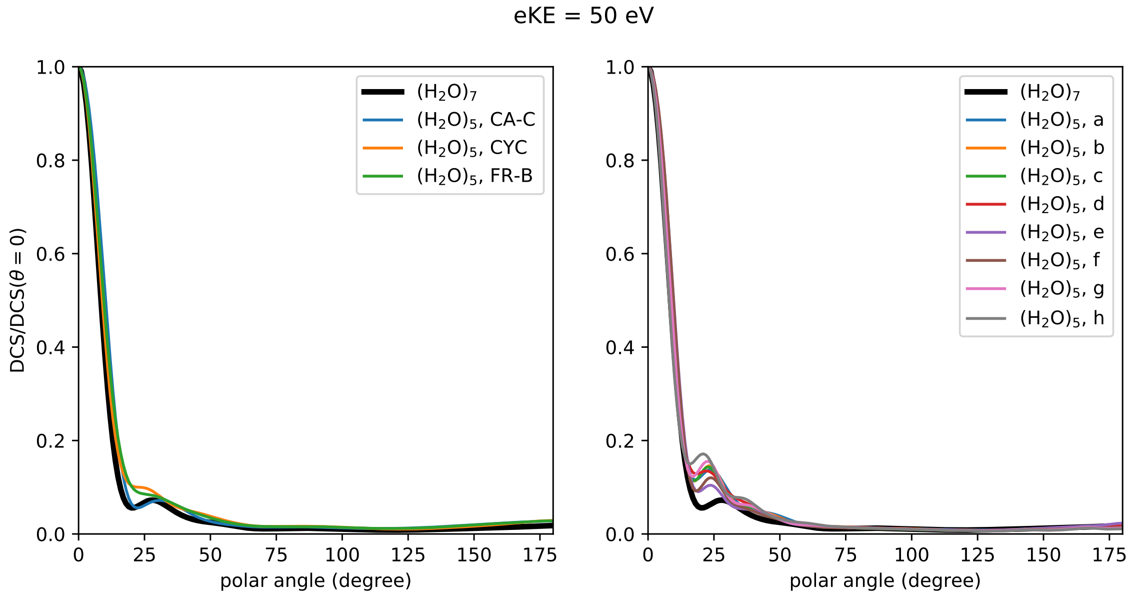


Figure S2: Left: Differential scattering cross sections (DCS) for three $(H_2O)_5$-clusters and the $(H_2O)_7$-cluster of lowest energy considered in [4]. Right: DCS for eight structures of $(H_2O)_5$-clusters considered in [5] for modeling experimental results of the first solvation shell of liquid water, as well as the DCS for the $(H_2O)_7$-cluster of lowest energy considered in [4]. The electron kinetic energy is eKE = 50 eV. The label of the structures is that used in the corresponding articles.

An additional test to check whether our cluster calculations provide a reasonable approximation for liquid-phase scattering is to compare the DCS for different cluster structures found in the *ab initio* calculations of [4] and for the structure of the first solvation shell of liquid water used to model the experimental results from X-ray absorption spectroscopy and X-ray Raman scattering.[5] The (scaled) DCS for the $(H_2O)_5$-clusters are shown in Figure S2 together with the (scaled) DCS for the $(H_2O)_7$-cluster that was used as approximation for the liquid-phase DCS in the simulations, for eKE = 50 eV. The left panel of Figure S2 compares the DCS for $(H_2O)_7$ with the DCS for three of the *ab initio* structures of $(H_2O)_5$ (see [4] for the structures; we use the labels of this article), while the right panel compares the DCS for $(H_2O)_7$ with the DCS for the structures that were used to model the first solvation shell of the liquid (see [5] for the structures; we use the labels of this article). From the picture, it is clear that there is some variation of the DCS of the $(H_2O)_5$-clusters. Both in the forward-scattering direction and for polar angles larger than 50 °, there is little difference between the scaled DCS for $(H_2O)_7$-cluster and those for the considered $(H_2O)_5$-clusters. For angles between ca. 15 ° and 50 ° the DCS for the $(H_2O)_5$-clusters are larger than that of $(H_2O)_7$ due to the finite size of the clusters. As seen in the convergence of the DCS when increasing the cluster size, shown in the left panel of Figure S1, we expect the relative DCS contribution to be small in this angular region for the liquid. Based on this comparison, we conclude that the DCS for the $(H_2O)_7$-cluster should be a reasonable approximation for the average DCS of liquid water, even if different solvation structures are present in the liquid.

## 2 Comments on the Monte-Carlo calculations

The assumptions made in the Monte-Carlo simulations are **(a)** that water up to the surface is modeled as a homogeneous and isotropic medium, **(b)** that the angular distribution of the electrons ionized from the oxygen 1s shell is similar to that of gas phase water, and **(c)** that ionization happens with equal probability everywhere inside the medium. Assumption (a) is necessary to obtain EMFP and IMFP values which correspond to their theoretical definitions, assumption (b) is made because neighboring water molecules only influence valence electrons but not the core electrons, and assumption (c) is justified because the absorption length of the radiation is much larger than the EAL [6]. Hence, trajectories originating from depths below the surface where the ionization probability is significantly reduced cannot reach the surface due to inelastic scattering.

Further details how the simulation works, as well as example files that show how the quantities considered in our article can be obtained, can be found on the website of the Python module `CLstunfti` that we developed for this work and that is available at `https://gitlab.com/axelschild/CLstunfti`.

# 3 Data for the calculation of the mean free paths

The effective attenuation lengths (EAL) were obtained from the experimental data of [7] by interpolation of the tabulated values. The parameters $\beta$ of the photoelectron angular distribution (PAD) were obtained by graphical extraction from the figure in [8] and subsequent interpolation. Table 1 lists all used parameters and the obtained values for the EMFP and $\langle N_{ela} \rangle$. The EMFP was determined with an accuracy of 0.01 nm and the $\langle N_{ela} \rangle$ with an accuracy of 0.05. This accuracy only characterizes the convergence and does not reflect the real accuracy of the values, which is less due to experimental uncertainties, the scarcity of experimental data for some eKE values and thus the interpolation error for the input data, as well as errors in the DCS due to the limited description of the electronic structures of the molecular clusters.

| eKE (eV) | EAL (nm) | $\beta_{gas}$ | $\beta_{liq}$ | EMFP (nm) | $\lambda_{ela}$ (nm) | $\langle N_{ela} \rangle$ | IMFP (nm) |
|---|---|---|---|---|---|---|---|
| 10 | 1.33 | 0.88 | 0.27 | 0.56 | 0.26 | 6.8 | 3.8 |
| 20 | 1.64 | 1.44 | 0.46 | 0.84 | 0.37 | 5.5 | 4.6 |
| 30 | 1.70 | 1.63 | 0.66 | 1.19 | 0.48 | 3.1 | 3.6 |
| 40 | 1.67 | 1.73 | 0.83 | 1.47 | 0.61 | 2.0 | 3.0 |
| 50 | 1.69 | 1.80 | 0.97 | 1.58 | 0.68 | 1.9 | 3.0 |
| 60 | 1.80 | 1.85 | 1.10 | 2.03 | 0.74 | 1.3 | 2.7 |
| 70 | 1.89 | 1.88 | 1.20 | 2.29 | 0.83 | 1.2 | 2.8 |
| 80 | 1.90 | 1.91 | 1.27 | 2.47 | 0.90 | 1.0 | 2.6 |
| 90 | 1.94 | 1.94 | 1.33 | 2.52 | 0.94 | 1.1 | 2.7 |
| 100 | 1.96 | 1.96 | 1.37 | 2.78 | 1.00 | 0.9 | 2.6 |
| 150 | 2.30 | 1.99 | 1.48 | 3.50 | 1.28 | 0.8 | 2.9 |
| 200 | 2.74 | 1.99 | 1.53 | 4.09 | 1.57 | 0.8 | 3.3 |
| 250 | 3.18 | 2.00 | 1.55 | 4.49 | 1.91 | 0.8 | 3.8 |
| 300 | 3.40 | 2.00 | 1.56 | 4.61 | 2.30 | 0.9 | 4.3 |

Table 1: Effective attenuation lengths (EAL) extracted from [7] and $\beta$-parameters for the photoelectron angular distribution of gas-phase water ($\beta_{gas}$) and of liquid water ($\beta_{liq}$, which is $\beta$ in the main article) extracted from [8], as well as the determined elastic mean free path (EMFP) and the average number of elastic scatterings $\langle N_{ela} \rangle$ for different values of the electron kinetic energy (eKE). Also given is the inelastic mean free path (IMFP = EMFP $\times \langle N_{ela} \rangle$). The table also contains the elastic mean free path $\lambda_{ela} = \frac{7}{\sigma n}$ obtained from the integrated cross section $\sigma$ for the heptamer cluster, where $n = 3.35 \times 10^{22}\,cm^{-3}$ is the number density of liquid water. *The accuracy of the numbers for the* EMFP, IMFP, *and* $\langle N_{ela} \rangle$ *in the table reflect only the numerical accuracy of the optimization procedure. Also, the values for the* EAL *and for* $\beta$ *were obtained by graphical extraction from experimental data that partially have a large uncertainty.*

We also investigated the uncertainty of the obtained results for the EMFP and $\langle N_{ela} \rangle$ by varying the input values taken from experiment. In particular, we made test calculations with an EAL changed by $\pm 0.3$ nm and $\beta_{liq}$ changed by $\pm 0.1$. The changes due to those variations are shown in Figure S3. It can be seen that the EMFP is rather sensitive to the target PAD and also somewhat sensitive to the EAL, while $\langle N_{ela} \rangle$ is comparably insensitive. In particular, $\langle N_{ela} \rangle$ does essentially not depend on the EAL but only influences the PAD. The independence of $\langle N_{ela} \rangle$ on the EAL can be understood as scale invariance of the model, i.e., a larger EAL corresponds to scaling all trajectories by a factor, hence EMFP and IMFP are also scaled by this factor but their ration, which is $\langle N_{ela} \rangle$, is unaffected. However, as the IMFP is the product of EMFP and $\langle N_{ela} \rangle$, it is also relatively sensitive to both the EAL and the PAD. This sensitivity indicates that good experimental values for the EAL and, in particular, for the PAD are necessary to obtain a reliable EMFP and IMFP.

Further tests of our results were made by comparison with the EMFP from [9] (corresponding to the integrated scattering cross sections for gas-phase water from [10]) and the IMFP from [11]. First, we note that the elastic mean free path calculated directly from the integrated DCS, given as $\lambda_{ela}$ in Table 1, converges to the EMFP of [9] with the eKE, i.e., to the EMFP expected from the gas-phase. This is also illustrated in the left panel of Figure S4. That the EMFP of the cluster converges to that of the gas-phase is expected for high eKE values, as the de-Broglie wavelength of the electron becomes very short and the electron-molecule collisions become core-penetrating.

Next, we investigated how the EAL and the PAD change if we use the EMFP from [9] and the IMFP from [11] as input values for the simulation. The resulting EAL is shown in the right panel of Figure S4, while the experimental one is shown in the left panel. The PAD and thus $\beta_{liq}$ change only very little with $\beta$ becoming slightly smaller (not shown). However, the EAL changes significantly, becoming much shorter than the measured values of [7]. Turning the table, we can use this computed EAL together with the experimental $\beta$-parameters to optimize the EMFP and IMFP. The result is a shift of EMFP and IMFP to smaller values (the average number of elastic scatterings is determined by $\beta$ and stays approximately constant) compared to what would be obtained with the experimental results for the EAL. This can be seen when comparing the left and right panel of Figure S4: In the left panel, the results are shown for the experimental EAL, while in the right panel the results are shown for the calculated EAL.

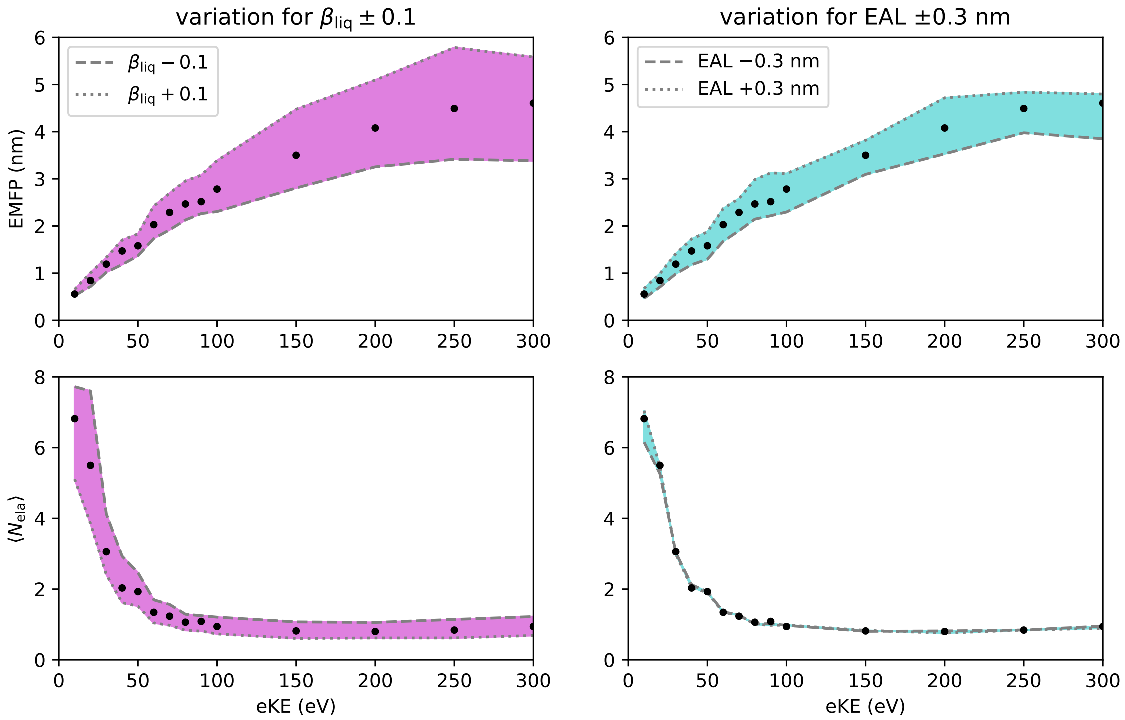


Figure S3: Variation of the elastic mean free path (EMFP) and the average number of elastic scatterings $\langle N_{ela} \rangle$ for a variation of the target parameters. The black line indicates the results obtained by optimizing the EMFP and $\langle N_{ela} \rangle$ to match the experimental target values. Left: Variation of the EMFP and of $\langle N_{ela} \rangle$ if the parameter $\beta_{liq}$ describing the photoelectron angular distribution of the liquid is changed from the target value by $\pm 0.1$, indicated as magenta area. Right: Variation of the EMFP and of $\langle N_{ela} \rangle$ if the effective attenuation length (EAL) is changed from the target value by $\pm 0.3$ nm, indicated as cyan area.

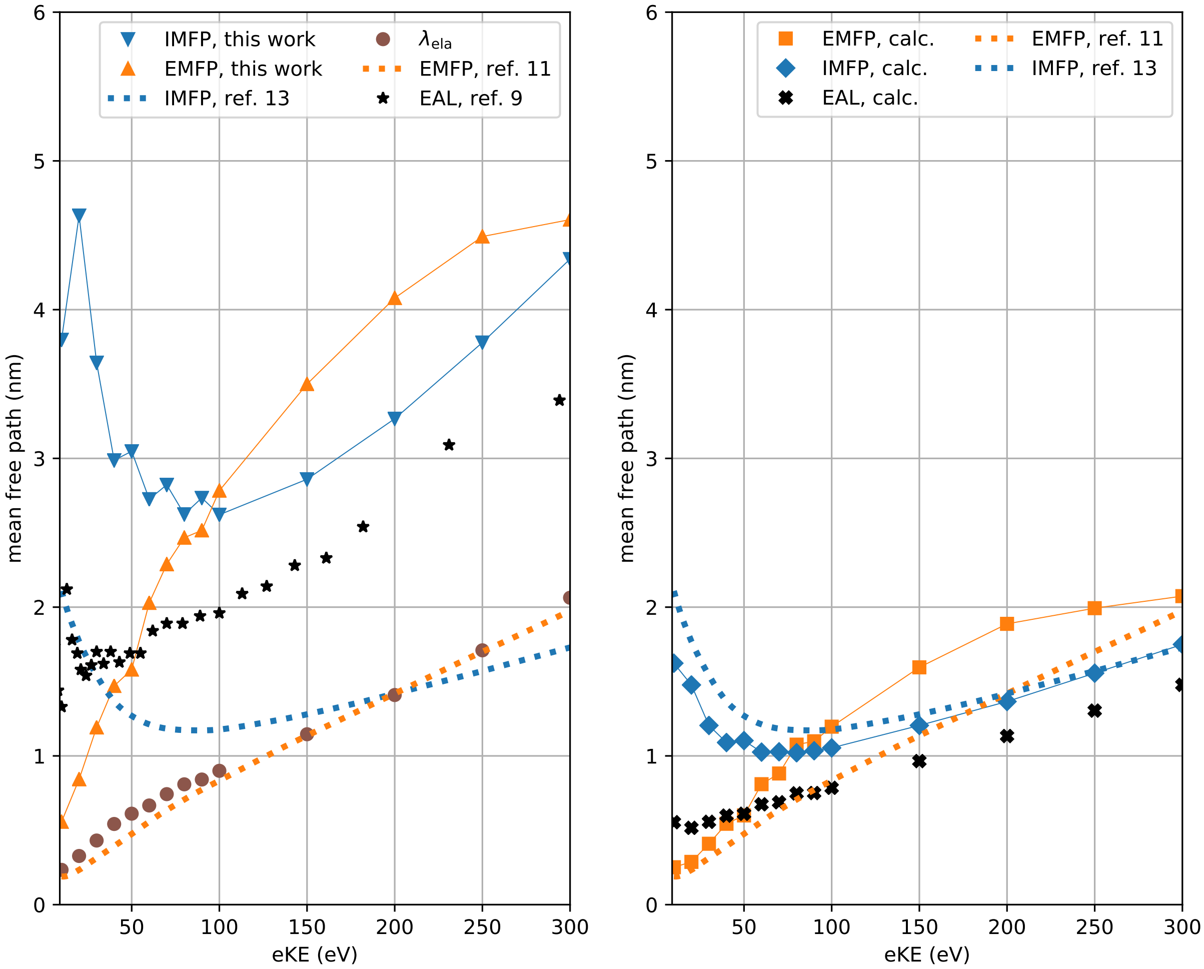


Figure S4: Left: Elastic and inelastic mean free path (EMFP, IMFP) obtained from our simulation when optimizing for the experimental photoelectron angular distribution (PAD) of [8] and the experimental effective attenuation length (EAL) of [7]. Shown is also the elastic mean free path $\lambda_{\mathrm{ela}}$ obtained from the total elastic cross section of the water heptamer cluster calculated with ePolyScat, the EMFP for gas-phase water from [10, 9], and the theoretical IMFP from [11]. Right: Taking the EMFP from [10, 9] and the IMFP from [11] as input for the simulations, the EAL shown as "EAL, calc." is obtained. By taking this EAL and the experimental PAD of [8] as input, we find "EMFP, calc." and "IMFP, calc." as optimal values from our simulations.

# 4 Further information

In [8], the average number of elastic scatterings $\langle \mathtt{N}_{\mathrm{ela}} \rangle$ was estimated by finding the number of scattering that are necessary to turn the measured gas-phase photoelectron angular distribution (PAD) into the measured liquid-phase PAD, for oxygen-1s ionization. For this purpose, the DCS $\mathtt{D}_{\mathrm{S}}(\theta)$ was approximated by a Gaussian function $\mathtt{D}_{\mathrm{S}}(\theta) \approx \mathtt{g}(\theta) \propto \mathtt{e}^{-\theta^2/(2\sigma^2)}$ with a variance $\sigma^2 = 17^\circ$ and convolutions were made of the gas-phase PAD with the DCS, until the liquid-phase PAD is obtained. The PAD $\mathtt{D}^{(\mathtt{n}+1)}(\theta)$ after $\mathtt{n}+1$ successive convolutions is then

$$\mathtt{D}^{(\mathtt{n}+1)}(\theta) = \int_0^{2\pi} \mathtt{D}^{(\mathtt{n})}(\theta')\mathtt{D}_{\mathrm{S}}(\theta - \theta')\sin(\theta')\mathtt{d}\theta'. \tag{1}$$

As explained in the main article, this approach is only valid in the bulk but neglects surface effects, which can impact the result drastically.

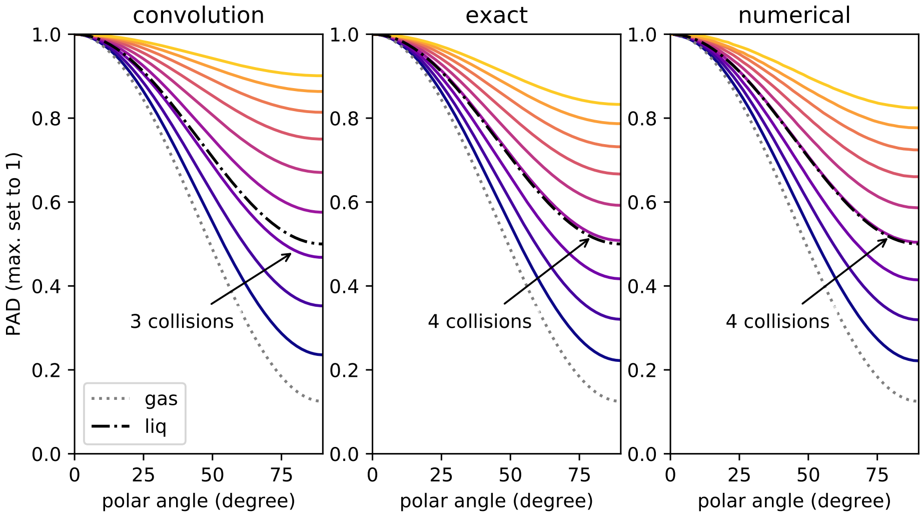


Figure S5: Photoelectron angular distribution (PAD) in the bulk (no surface): Dotted line is the gas-phase PAD (the PAD after ionization), dash-dotted line is the measured PAD after the electrons have left the liquid. Each successive solid line above the gas-phase-PAD is the PAD after one additional scattering. Left: Results obtained from a convolution using (1) (incorrect). Center: Exact result using (2). Right: PAD computed with our simulation code.

However, even in the bulk, (1) is only true for two-dimensional problems. For three-dimensional scattering, the formula to obtain the PAD after $\mathtt{n}+1$ successive scatterings is

$$\mathtt{D}^{(\mathtt{n}+1)}(\theta) = \int_0^{\pi}\int_0^{2\pi} \mathtt{D}^{(\mathtt{n})}(\vartheta)\mathtt{D}_{\mathrm{S}}(\vartheta')\sin(\vartheta)\,\mathtt{d}\vartheta\mathtt{d}\varphi \tag{2}$$

with

$$\cos\vartheta' = \cos(\vartheta)\cos(\theta) + \cos(\varphi)\sin(\vartheta)\sin(\theta). \tag{3}$$

We tested the difference between using (1) and (2) for an eKE of 20 eV. The results is shown in Figure S5. Using (1), ca. three scatterings are needed to turn the gas-phase PAD into the liquid-phase PAD, while the exact formula (2) shows that ca. four scatterings are necessary. However, the inclusion of surface effects has a much larger impact on the results than using (1) instead of (2), as ca. ten collisions are needed would then be necessary because electrons starting close to the surface have a lower probability to scatter than those in the bulk. This is shown in the main article in Figure 3.

## References


[1] F. A. Gianturco, R. R. Lucchese, and N. Sanna. Calculation of low-energy elastic cross sections for electron-$CF_4$ scattering. *The Journal of Chemical Physics*, 100(9):6464–6471, 1994.

[2] Alexandra P. P. Natalense and Robert R. Lucchese. Cross section and asymmetry parameter calculation for sulfur 1s photoionization of $SF_6$. *The Journal of Chemical Physics*, 111(12):5344–5348, 1999.

[3] M. J. Frisch, G. W. Trucks, H. B. Schlegel, G. E. Scuseria, M. A. Robb, J. R. Cheeseman, G. Scalmani, V. Barone, B. Mennucci, G. A. Petersson, H. Nakatsuji, M. Caricato, X. Li, H. P. Hratchian, A. F. Izmaylov, J. Bloino, G. Zheng, J. L. Sonnenberg, M. Hada, M. Ehara, K. Toyota, R. Fukuda, J. Hasegawa, M. Ishida, T. Nakajima, Y. Honda, O. Kitao, H. Nakai, T. Vreven, J. A. Montgomery, Jr., J. E. Peralta, F. Ogliaro, M. Bearpark, J. J. Heyd, E. Brothers, K. N. Kudin, V. N. Staroverov, T. Keith, R. Kobayashi, J. Normand, K. Raghavachari, A. Rendell, J. C. Burant, S. S. Iyengar, J. Tomasi, M. Cossi, N. Rega, J. M. Millam, M. Klene, J. E. Knox, J. B. Cross, V. Bakken, C. Adamo, J. Jaramillo, R. Gomperts, R. E. Stratmann, O. Yazyev, A. J. Austin, R. Cammi, C. Pomelli, J. W. Ochterski, R. L. Martin, K. Morokuma, V. G. Zakrzewski, G. A. Voth, P. Salvador, J. J. Dannenberg, S. Dapprich, A. D. Daniels, O. Farkas, J. B. Foresman, J. V. Ortiz, J. Cioslowski, and D. J. Fox. Gaussian 09 Revision D.01, 2013. Gaussian Inc. Wallingford CT.

[4] Berhane Temelso, Kaye A. Archer, and George C. Shields. Benchmark Structures and Binding Energies of Small Water Clusters with Anharmonicity Corrections. *The Journal of Physical Chemistry A*, 115(43):12034–12046, 2011. PMID: 21910428.

[5] Ph. Wernet, D. Nordlund, U. Bergmann, M. Cavalleri, M. Odelius, H. Ogasawara, L. Å. Näslund, T. K. Hirsch, L. Ojamäe, P. Glatzel, L. G. M. Pettersson, and A. Nilsson. The structure of the first coordination shell in liquid water. *Science*, 304(5673):995–999, 2004.

[6] Hisashi Hayashi and Nozomu Hiraoka. Accurate Measurements of Dielectric and Optical Functions of Liquid Water and Liquid Benzene in the VUV Region (1-100 eV) Using Small-Angle Inelastic X-ray Scattering. *The Journal of Physical Chemistry B*, 119(17):5609–5623, 2015. PMID: 25835527.

[7] Yoshi-Ichi Suzuki, Kiyoshi Nishizawa, Naoya Kurahashi, and Toshinori Suzuki. Effective attenuation length of an electron in liquid water between 10 and 600 eV. *Phys. Rev. E*, 90:010302, Jul 2014.

[8] Stephan Thürmer, Robert Seidel, Manfred Faubel, Wolfgang Eberhardt, John C. Hemminger, Stephen E. Bradforth, and Bernd Winter. Photoelectron Angular Distributions from Liquid Water: Effects of Electron Scattering. *Phys. Rev. Lett.*, 111:173005, Oct 2013.

[9] H. Tomita, M. Kai, T. Kusama, and A. Ito. Monte carlo simulation of physicochemical processes of liquid water radiolysis. *Radiation and Environmental Biophysics*, 36(2):105–116, Jul 1997.

[10] T. D. Märk, Y. Hatano, and F. Linder. Electron collision cross sections. In *Atomic and molecular data for radiotherapy and radiation research*. IAEA, Vienna, 1995.

[11] Hieu T Nguyen-Truong. Low-energy electron inelastic mean free paths for liquid water. *Journal of Physics: Condensed Matter*, 30(15):155101, 2018.
